# Supplementary material for: Prototype-Guided Diffusion for Digital Pathology: Achieving Foundation Model Performance with Minimal Clinical Data
Source: arXiv:2504.12351 source file (2025-04-15)
Supplement: Supplementary file 1 [file X_suppl.tex]

\clearpage
\setcounter{page}{1}
\maketitlesupplementary
\section{Datasets}
We provide descriptions of the datasets
used for the downstream experiments.

\textbf{NSCLC} For the non-small cell lung carcinoma (NSCLC) subtyping task, we utilize H\&E WSIs from the PLCO dataset to classify cases of lung adenocarcinoma (LUAD) and lung squamous cell carcinoma (LUSC). The PLCO cohort contains 589 slides from 274 patients (LUAD: 171, LUSC: 103).
We perform a patient-level, label-stratified split of both cohorts into training, validation, and test sets with a 70:10:20 ratio. Performance was evaluated using AUCROC and F1-Score.

We also ran a lung cancer survival task using the same PLCO lung cohort. Mortality status from the PLCO study data is used to determine survival, censorship, and duration of survival for this dataset. Out of 274 participants, 213 survived. We performed a patient-level, label-stratified split into training, validation, and test sets with a 70:10:20 ratio. Performance was evaluated using the c-index.

\textbf{PANDA} For the prostate cancer ISUP grading task, we utilized 10,616 core needle biopsy cases collected from Karolinska Institute and Radboud University Medical Center. All biopsy WSIs were obtained from the Prostate Cancer Grade Assessment (PANDA) challenge. Each biopsy is assigned an ISUP grade on a scale from 1 to 5 if cancerous, while benign biopsies receive a label of 0, resulting in a six-class classification problem. The class distribution is as follows: class 0  (2892), class 1  (2666), class 2  (1343), class 3  (1242), class 4  (1249), and class 5 (1224). Patient identification information was not provided in the dataset, so patient-level splits could not be created.  Instead, we perform a label-stratified split into training, validation, and test sets with a 70:10:20 ratio. Performance was evaluated using AUCROC and macro F1-Score.

\textbf{Camelyon16} We used the CAMELYON16 dataset, which includes 397 WSIs from sentinel lymph node biopsies, to detect metastases in breast cancer patients. Metastases are categorized into three classes—'negative' (237), 'micro' (80), and 'macro' (80)—making this a three-class classification problem. Patient identification information was not provided in the dataset, so patient-level splits could not be created. Instead, we perform a label-stratified split into training, validation, and test sets with a 70:10:20 ratio. Performance was evaluated using AUCROC and macro F1-Score.

\textbf{UBC-OCEAN} For ovarian cancer subtype classification, we utilized 513 biopsy samples from the UBC ovarian cancer subtype classification and outlier detection (UBC-OCEAN) competition. Each sample is assigned one out of five histological subtypes of ovarian cancer: class 0 (217), class 1 (42), class 2 (119),  class 3 (94), and class 4 (41). Patient identification information was not provided in the dataset, so patient-level splits could not be created. Instead, we perform a label-stratified split into training, validation, and test sets with a 70:10:20 ratio. Performance was evaluated using AUCROC and macro F1-Score.

\textbf{Breast} For the breast cancer subtyping task, we used the PLCO Breast dataset. The PLCO cohort consists of 1768 slides from 867 patients. Each sample is categorized into one of three classes - 'lobular' (104), 'ductal' (657), and 'other' (106). We perform patient-level, label-stratified split into training, validation, and test sets with a 70:10:20 ratio. Performance was evaluated using AUCROC and macro F1-Score.

We use the same dataset for breast cancer survival tasks. Mortality status from the PLCO study data is used to determine survival, censorship, and duration of survival. Out of 867 participants, 552 survived. The TCGA-BRCA dataset consists of 1267 WSIs spanning 1042 patients, with 963 surviving based on disease-specific survival (DSS) status. We perform a patient-level, label-stratified split for both datasets into training, validation, and test sets with a 70:10:20 ratio. Performance was evaluated using the c-index.

\textbf{Prostate}
For our prostate cancer biochemical recurrence (BCR) tasks, we use an in-house dataset of radical prostatectomy whole-mount WSIs. The in-house dataset spans 161 patients, with one whole-mount WSI selected per patient based on pathology reports. The ratio of patients without BCR versus those with BCR is 135:26. The Gleason grading breakdown of this dataset is: 74 - 3+4 cases, 46 - 4+3 cases, 20 - 4+5 cases, 13 - 3+3 cases, 6 - 4+4 cases, 1 - 3+5 case, and 1 - 5+4 case. We perform a patient-level, label-stratified split into training, validation, and test sets with a 70:10:20 ratio. Performance was evaluated using the c-index.

\section{Clustering}
 We performed clustering within each tissue type, varying $k$ across a range of values. To determine the optimal number of clusters, we calculated the within-cluster sum of squares (WCSS) and applied the elbow method. The corresponding elbow plots are shown in Figure \ref{fig:clustering}).

\begin{figure*}[]
    \centering
    \includegraphics[width=\linewidth]{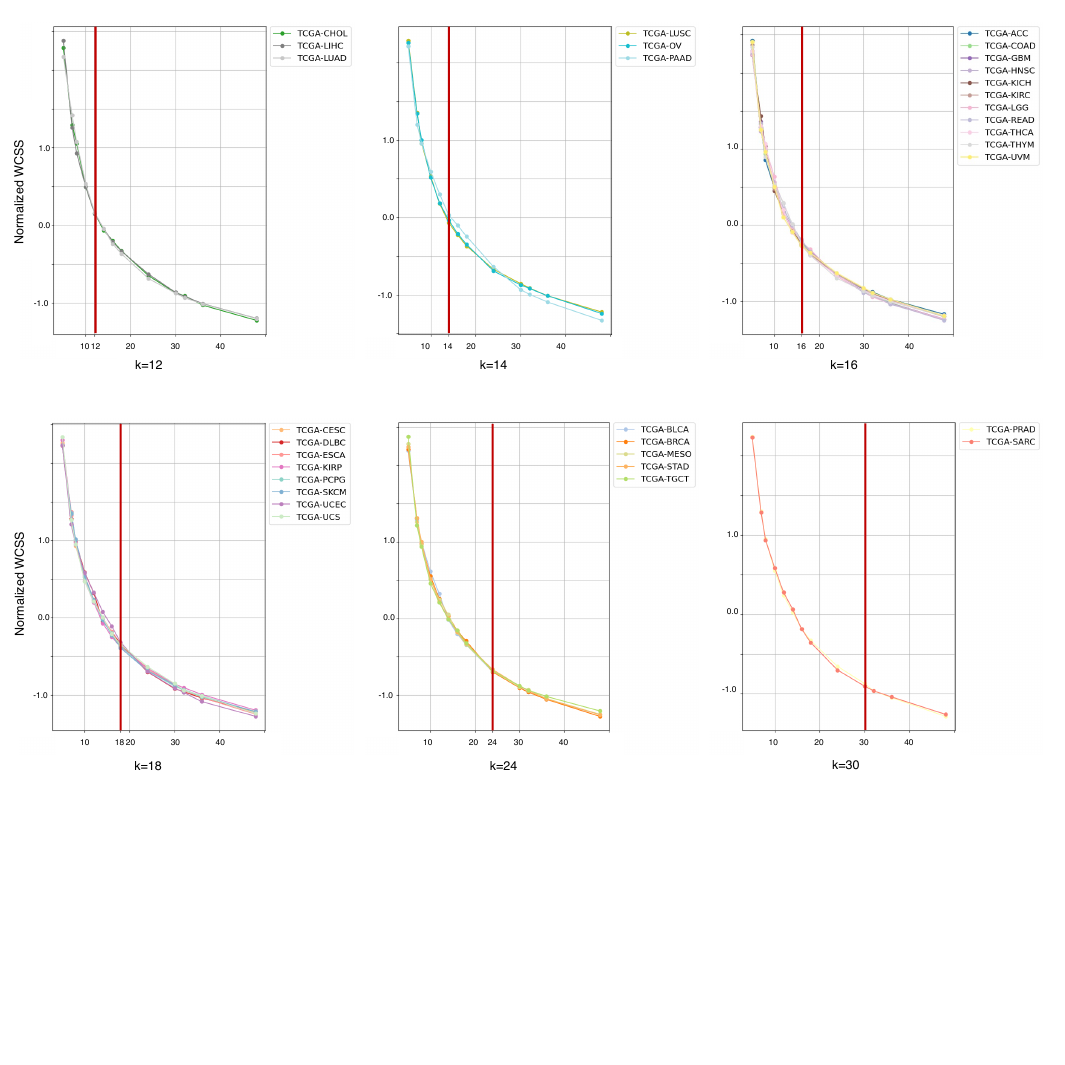} %
    \caption{Within-Cluster Sum of Squares (WCSS) Elbow Plots Across Values of k. Plots are grouped by k, chosen for each tissue type.}
    \label{fig:clustering} % Reference label
\end{figure*}

\section{Model and training}
For downstream training, we employ a weight decay of $1 \times 10^{-5}$ and use the AdamW optimizer with a learning rate of $1 \times 10^{-4}$, along with a cosine decay scheduler. For the slide classification experiments, we utilized a cross-entropy loss. We employed early stopping if the validation loss failed to improve over ten consecutive epochs with a total training epochs of 20. For survival prediction experiments, we used negative log-likelihood loss (NLL).

\textbf{ABMIL downstream architecture:} ABMIL architecture used in the downstream experiments consists of three components. First, a 2-layer MLP with 256 or 512 hidden units, layer normalization, ReLu activation, and 0.25 dropout. This is followed by a gated-attention network consisting of 2-layer
MLP, with Sigmoid and Tanh activation, respectively, and 0.25 dropout. Finally, a post-attention linear classification layer with 256 or 512 hidden units is applied.
